# Supplementary material for: Developments in NuWro Monte Carlo generator
Source: arXiv:2501.11470 source file (2025-01-22)
Supplement: Supplementary file 1 [file appendices.tex]

\appendix
\section{\label{app:one} Algorithm of new MC MEC model}
